# Supplementary material for: Deep Fashion3D: A Dataset and Benchmark for 3D Garment Reconstruction from Single Images
Source: arXiv:2003.12753 source file (2020-07-04)
Supplement: Supplementary file 1 [file supplemented_materials.tex]

In this supplemental material, we provide more results and analysis in the following aspects: 1) more comparisons with the state-of-the-art methods; 2) more results of 3DFashionNet; 3) more implementation details; 4) visualization of more sample point clouds of Fashion3D dataset.
%Due to space restrictions, some important details are omitted from the main part of the paper. Here in this section, we will present the omitted details from following five aspects:

\nothing{
\begin{itemize}
	\item Implementation details, loss functions and hyper parameters
	\item The limitations of Garment Net's parameter space
	\item More comparison between our method and the state of the arts 
	\item A more detailed dive into our Fashion3D dataset
	\item More results generated using our proposed model
\end{itemize}
}

\section{More Comparisons}
In the main paper, we only show the comparisons with the state-of-the-arts on the task of single-view garment in the front view. To provide more comprehensive evaluations, we further visualize the results in side views in Figure \ref{fig:qualiResultsLeft}. 

\begin{figure}[h]
\centering
\includegraphics[width=1\linewidth]{figs/supplement/mgn_modified_final.pdf}
% ground truth point cloud, or the image rendered
\caption{
Comparisons between our method and Multi-Garment Net. (a) Input images; (b) Our results (c) Results generated by Multi-Garment net; (d) Ground-truth point clouds.}
\label{fig:garnetlimit}
\end{figure}

\begin{figure*}[h]
\centering
\includegraphics[width=0.95\linewidth]{figs/supplement/demo5.pdf}
\caption{Comparisons with other state-of-the-art methods visualized in different views. Given an input image (leftmost), we show the reconstruction results by different approaches. (a) 3D-R2N2 \cite{choy20163d}; (b) SketchModeling \cite{lun20173d}; (c) PointSetGen \cite{Fan_2017_CVPR}; (d) Pixel2Mesh \cite{wang2018pixel2mesh}; (e) AtlasNet-Sphere \cite{groueix2018}; (f) AtlasNet-Patch25 \cite{groueix2018}; (g) Ours and (h) Ground truth.}
\label{fig:qualiResultsLeft}
\end{figure*}

\paragraph{Comparisons with Multi-Garment Net~\cite{bhatnagar2019multi}.}

We also compare the reconstructed meshes generated by our model with that of the state-of-the-art garment reconstruction method -- Multi-Garment Net (MGN) in Figure~\ref{fig:garnetlimit}. 
The results produced by MGN is obtained by optimizing the garment parameters to fit the ground-truth point cloud, while our method infers the mesh directly from the input single image. 
As MGN can only model limited cloth categories, it fails to reconstruct the dress and vest models as shown in the first and second row in Figure~\ref{fig:garnetlimit}.
In addition, the clothing wrinkles reconstructed by MGN (last row of Figure~\ref{fig:garnetlimit}) deviate greatly from the ground truth while our approach is able to generate plausible results.
The reason is that MGN relies on a pre-trained parametric model that has limited expressiveness and thus cannot handle large varieties of dynamic clothing deformations.
In contrast, our approach is blendshape-free and is trained on a large amount of real deformations. 
%It is plain to see that the parameter space of Multi-Garment Net fails to express the complicated wrinkles on the garments in our 3D garment data set. 
%Moreover, it is obvious that the parameter space proposed in Multi-Garment Net encounters difficulties when facing various real world garment categories including dress, vest, skirts, etc.
%representing various 

%\vspace{-2mm} 

\section{More Results}
%This subsection shows more results on our proposed Fashion3D dataset. The %meshes are generated by 3DFashionNet with the images in
In this section, we show more results generated by our 3DFashionNet in Figure~\ref{fig:more_results}. 
Note that the images adopted for testing are rendered using novel point clouds from Fashion3D that were not seen during training. 
%Note that there is no overlap between the garments used for testing and the garments used for training.

\begin{figure*}[ht]
\centering
\includegraphics[width=0.95\linewidth]{figs/supplement/more_results_kai.pdf}
\caption{More single-view reconstruction results generated by 3DFashionNet. For each group of results, we show the input images and reconstructed models in two different views from left to right.}
\label{fig:more_results}
\end{figure*}

\section{Implementation Details}
In the main paper, we briefly introduce the losses adopted to train our proposed 3DFashionNet. In this section, we will describe the loss functions as well as the hyper parameters of two cascaded stages with more details.

\paragraph{Feature Line Fitting Stage.} 
As mentioned in the main paper, a novel feature line loss $\mathcal{L}_{line}$\ as well as the edge length regularization loss $\mathcal{L}_{fed}$\ are adopted to guide the feature line synthesis while reducing the zigzag artifacts:
\begin{center}
    $\mathcal{L}_{fitting}$\ = $\mathcal{L}_{line}$\ + $\lambda_{fed}$\ $\mathcal{L}_{fed}$,\
\end{center}

\noindent where $\lambda_{fed}$\ is set to 1 for the first cascade stage and 0.5 for the second one.

\paragraph{Surface Refinement Stage.} 
In the surface refinement stage, apart from the feature line loss $\mathcal{L}_{line}$\ and edge length regularization loss $\mathcal{L}_{fed}$\ which are adopted for training the feature line fitting stage, Chamfer loss $\mathcal{L}_{chm}$, normal loss $\mathcal{L}_{nor}$, mesh edge loss $\mathcal{L}_{med}$, and Laplacian loss $\mathcal{L}_{lap}$ defined in Pix2Mesh\cite{wang2018pixel2mesh} are also employed:
\begin{center}
    $\mathcal{L}_{refine}$\ = $\mathcal{L}_{chm}$\ + $\lambda_{nor}$\ $\mathcal{L}_{nor}$\ + $\lambda_{lap}$\ $\mathcal{L}_{lap}$\ + $\lambda_{med}$\ $\mathcal{L}_{med}$\ + $\lambda_{line}$\ $\mathcal{L}_{line}$\ + $\lambda_{fed}$\ $\mathcal{L}_{fed}$,\
\end{center}

\noindent where $\lambda_{nor}$\ , $\lambda_{lap}$\ , $\lambda_{med}$\, $\lambda_{line}$\ , $\lambda_{fed}$\ are set to $1.6 \times 10^{-4}$, 1, 0.5, 1, and 0.5 respectively.
\section{Sample Point Clouds of Fashion3D}
In Figure \ref{fig:qualiResultsLeft}., we show more sample point clouds of our Fashion3D dataset in multiple views.

\begin{figure*}[ht]
\centering
\includegraphics[width=0.95\linewidth]{figs/supplement/dataset_point_clouds.pdf}
\caption{Sample point clouds of our Fashion3D dataset visualized from multiple views.}
\label{fig:supppointclouds}
\end{figure*}
