# Supplementary material for: Deep Fashion3D: A Dataset and Benchmark for 3D Garment Reconstruction from Single Images
Source: arXiv:2003.12753 source file (2020-07-04)
Supplement: Supplementary file 2 [file suppl_dataset.tex]

\section{Sample Point Clouds of Fashion3D}
In Figure \ref{fig:qualiResultsLeft}., we show more sample point clouds of our Fashion3D dataset in multiple views.

\begin{figure*}[ht]
\centering
\includegraphics[width=0.95\linewidth]{figs/supplement/dataset_point_clouds.pdf}
\caption{Sample point clouds of our Fashion3D dataset visualized from multiple views.}
\label{fig:supppointclouds}
\end{figure*}
