# Supplementary material for: Deep Fashion3D: A Dataset and Benchmark for 3D Garment Reconstruction from Single Images
Source: arXiv:2003.12753 source file (2020-07-04)
Supplement: Supplementary file 3 [file suppl_impDetails.tex]

\section{Implementation Details}
In the main paper, we briefly introduce the losses adopted to train our proposed 3DFashionNet. In this section, we will describe the loss functions as well as the hyper parameters of two cascaded stages with more details.

\paragraph{Feature Line Fitting Stage.} 
As mentioned in the main paper, a novel feature line loss $\mathcal{L}_{line}$\ as well as the edge length regularization loss $\mathcal{L}_{fed}$\ are adopted to guide the feature line synthesis while reducing the zigzag artifacts:
\begin{center}
    $\mathcal{L}_{fitting}$\ = $\mathcal{L}_{line}$\ + $\lambda_{fed}$\ $\mathcal{L}_{fed}$,\
\end{center}

\noindent where $\lambda_{fed}$\ is set to 1 for the first cascade stage and 0.5 for the second one.

\paragraph{Surface Refinement Stage.} 
In the surface refinement stage, apart from the feature line loss $\mathcal{L}_{line}$\ and edge length regularization loss $\mathcal{L}_{fed}$\ which are adopted for training the feature line fitting stage, Chamfer loss $\mathcal{L}_{chm}$, normal loss $\mathcal{L}_{nor}$, mesh edge loss $\mathcal{L}_{med}$, and Laplacian loss $\mathcal{L}_{lap}$ defined in Pix2Mesh\cite{wang2018pixel2mesh} are also employed:
\begin{center}
    $\mathcal{L}_{refine}$\ = $\mathcal{L}_{chm}$\ + $\lambda_{nor}$\ $\mathcal{L}_{nor}$\ + $\lambda_{lap}$\ $\mathcal{L}_{lap}$\ + $\lambda_{med}$\ $\mathcal{L}_{med}$\ + $\lambda_{line}$\ $\mathcal{L}_{line}$\ + $\lambda_{fed}$\ $\mathcal{L}_{fed}$,\
\end{center}

\noindent where $\lambda_{nor}$\ , $\lambda_{lap}$\ , $\lambda_{med}$\, $\lambda_{line}$\ , $\lambda_{fed}$\ are set to $1.6 \times 10^{-4}$, 1, 0.5, 1, and 0.5 respectively.
