# Supplementary material for: Deep Fashion3D: A Dataset and Benchmark for 3D Garment Reconstruction from Single Images
Source: arXiv:2003.12753 source file (2020-07-04)
Supplement: Supplementary file 4 [file suppl_moreCompare.tex]

\section{More Comparisons}
In the main paper, we only show the comparisons with the state-of-the-arts on the task of single-view garment in the front view. To provide more comprehensive evaluations, we further visualize the results in side views in Figure \ref{fig:qualiResultsLeft}. 

\begin{figure}[h]
\centering
\includegraphics[width=1\linewidth]{figs/supplement/mgn_modified_final.pdf}
% ground truth point cloud, or the image rendered
\caption{
Comparisons between our method and Multi-Garment Net. (a) Input images; (b) Our results (c) Results generated by Multi-Garment net; (d) Ground-truth point clouds.}
\label{fig:garnetlimit}
\end{figure}

\begin{figure*}[h]
\centering
\includegraphics[width=0.95\linewidth]{figs/supplement/demo5.pdf}
\caption{Comparisons with other state-of-the-art methods visualized in different views. Given an input image (leftmost), we show the reconstruction results by different approaches. (a) 3D-R2N2 \cite{choy20163d}; (b) SketchModeling \cite{lun20173d}; (c) PointSetGen \cite{Fan_2017_CVPR}; (d) Pixel2Mesh \cite{wang2018pixel2mesh}; (e) AtlasNet-Sphere \cite{groueix2018}; (f) AtlasNet-Patch25 \cite{groueix2018}; (g) Ours and (h) Ground truth.}
\label{fig:qualiResultsLeft}
\end{figure*}

\paragraph{Comparisons with Multi-Garment Net~\cite{bhatnagar2019multi}.}

We also compare the reconstructed meshes generated by our model with that of the state-of-the-art garment reconstruction method -- Multi-Garment Net (MGN) in Figure~\ref{fig:garnetlimit}. 
The results produced by MGN is obtained by optimizing the garment parameters to fit the ground-truth point cloud, while our method infers the mesh directly from the input single image. 
As MGN can only model limited cloth categories, it fails to reconstruct the dress and vest models as shown in the first and second row in Figure~\ref{fig:garnetlimit}.
In addition, the clothing wrinkles reconstructed by MGN (last row of Figure~\ref{fig:garnetlimit}) deviate greatly from the ground truth while our approach is able to generate plausible results.
The reason is that MGN relies on a pre-trained parametric model that has limited expressiveness and thus cannot handle large varieties of dynamic clothing deformations.
In contrast, our approach is blendshape-free and is trained on a large amount of real deformations. 
%It is plain to see that the parameter space of Multi-Garment Net fails to express the complicated wrinkles on the garments in our 3D garment data set. 
%Moreover, it is obvious that the parameter space proposed in Multi-Garment Net encounters difficulties when facing various real world garment categories including dress, vest, skirts, etc.
%representing various 

%\vspace{-2mm} 
