# Supplementary material for: Deep Fashion3D: A Dataset and Benchmark for 3D Garment Reconstruction from Single Images
Source: arXiv:2003.12753 source file (2020-07-04)
Supplement: Supplementary file 5 [file suppl_moreResults.tex]

\section{More Results}
%This subsection shows more results on our proposed Fashion3D dataset. The %meshes are generated by 3DFashionNet with the images in
In this section, we show more results generated by our 3DFashionNet in Figure~\ref{fig:more_results}. 
Note that the images adopted for testing are rendered using novel point clouds from Fashion3D that were not seen during training. 
%Note that there is no overlap between the garments used for testing and the garments used for training.

\begin{figure*}[ht]
\centering
\includegraphics[width=0.95\linewidth]{figs/supplement/more_results_kai.pdf}
\caption{More single-view reconstruction results generated by 3DFashionNet. For each group of results, we show the input images and reconstructed models in two different views from left to right.}
\label{fig:more_results}
\end{figure*}
